# Supplementary material for: Relaxation Dynamics of Disordered Spin Chains: Localization and the Existence of a Stationary State
Source: arXiv:1206.4787 ancillary file (2012-12-20)
Supplement: Supplementary file 1 [file sm.pdf]

# Relaxation Dynamics of Disordered Spin Chains: Localization and the Existence of a Stationary State - Supplementary Material

Simone Ziraldo[1,2], Alessandro Silva[3], Giuseppe E. Santoro[1,2,3]
[1] *SISSA, Via Bonomea 265, I-34136 Trieste, Italy*
[2] *CNR-IOM Democritos National Simulation Center, Via Bonomea 265, I-34136 Trieste, Italy*
[3] *International Centre for Theoretical Physics (ICTP), P.O.Box 586, I-34014 Trieste, Italy*

## QUENCH TO A CLEAN XX CHAIN FINAL $\hat{H}$

When the final eigenstates are extended the value of $\delta^2_{j_1 j_2}$ goes to zero in the thermodynamic limit. In the particular case in which the final $\hat{H}$ is translationally invariant, we have to take care of the degeneracies $k$, $-k$, where $k$ is the momentum, and of particle-hole symmetry, which were not taken into account in the general derivation of the expression for $\delta^2_{j_1 j_2}$ (Eq. (4) of the main text). In this case the time-average of the single-fermion Green's functions becomes:

$$\overline{G_{j_1 j_2}(t)} = \sum_k u^*_{j_1 k} u_{j_2 k} \langle\psi_0| \hat{c}^\dagger_k \hat{c}_k |\psi_0\rangle + u^*_{j_1 k} u_{j_2 -k} \langle\psi_0| \hat{c}^\dagger_k \hat{c}_{-k} |\psi_0\rangle \tag{1}$$

where $u_{jk} = \exp(ikj)/\sqrt{L}$ is the plane wave with momentum $k$ and the second term is due to the degeneracy $k$, $-k$. The time-fluctuations of $G_{j_1 j_2}(t)$ is then equal to:

$$G_{j_1 j_2}(t) - \overline{G_{j_1 j_2}(t)} = {\sum_{k_1 k_2}}' e^{i\epsilon_{k_1} t} e^{-i\epsilon_{k_2} t} u^*_{j_1 k_1} u_{j_2 k_2} \langle\psi_0| \hat{c}^\dagger_{k_1} \hat{c}_{k_2} |\psi_0\rangle$$

where the prime indicates that the summation is over all the $k_1$ and $k_2$ with $|k_1| \neq |k_2|$. Using this expression and the definition of $\delta^2_{j_1 j_2}$ we have:

$$\delta^2_{j_1 j_2} = {\sum_{k_1 k_2}}' {\sum_{k_3 k_4}}' \Delta(k_1, k_2, k_3, k_4) u^*_{j_1 k_1} u_{j_2 k_2} u_{j_1 k_3} u^*_{j_2 k_4} \langle\psi_0| \hat{c}^\dagger_{k_1} \hat{c}_{k_2} |\psi_0\rangle \langle\psi_0| \hat{c}^\dagger_{k_3} \hat{c}_{k_4} |\psi_0\rangle^* \tag{2}$$

where $\Delta(k_1, k_2, k_3, k_4) \equiv \overline{e^{i(\epsilon_{k_1} - \epsilon_{k_2} - \epsilon_{k_3} + \epsilon_{k_4})t}}$ is one when $\epsilon_{k_1} - \epsilon_{k_2} - \epsilon_{k_3} + \epsilon_{k_4} = 0$ and zero otherwise. Using the fact that $|u_{jk}| = 1/\sqrt{L}$ we have:

$$\begin{aligned}
\delta^2_{j_1 j_2} &\leq \frac{1}{L^2} {\sum_{k_1 k_2}}' {\sum_{k_3 k_4}}' \Delta(k_1, k_2, k_3, k_4) \left|\langle\psi_0| \hat{c}^\dagger_{k_1} \hat{c}_{k_2} |\psi_0\rangle\right| \left|\langle\psi_0| \hat{c}^\dagger_{k_3} \hat{c}_{k_4} |\psi_0\rangle\right| \\
&\leq \frac{1}{2L^2} {\sum_{k_1 k_2}}' {\sum_{k_3 k_4}}' \Delta(k_1, k_2, k_3, k_4) \left( \left|\langle\psi_0| \hat{c}^\dagger_{k_1} \hat{c}_{k_2} |\psi_0\rangle\right|^2 + \left|\langle\psi_0| \hat{c}^\dagger_{k_3} \hat{c}_{k_4} |\psi_0\rangle\right|^2 \right) \\
&\leq \frac{1}{L^2} {\sum_{k_1 k_2}}' \left( \left|\langle\psi_0| \hat{c}^\dagger_{k_1} \hat{c}_{k_2} |\psi_0\rangle\right|^2 {\sum_{k_3 k_4}}' \Delta(k_1, k_2, k_3, k_4) \right)
\end{aligned} \tag{3}$$

where (in the second inequality) we used that, if $a$ and $b$ are real numbers then $2ab \leq a^2 + b^2$, and (in the third inequality) that $\Delta(k_1, k_2, k_3, k_4) = \Delta(k_3, k_4, k_1, k_2)$. Once fixed $k_1$ and $k_2$, with $|k_1| \neq |k_2|$, the inner sum is 4 when $|k_1| = \pi - |k_2|$, and 8 in the other cases [1] and therefore:

$$\delta^2_{j_1 j_2} \leq \frac{8}{L^2} \sum_{k_1 k_2} \left|\langle\psi_0| \hat{c}^\dagger_{k_1} \hat{c}_{k_2} |\psi_0\rangle\right|^2 \tag{4}$$

where we also added the (positive) terms $|k_1| = |k_2|$ to the sum. Expressing the operators $\hat{c}^\dagger_k$ and $\hat{c}_k$ in terms of the fermions of the initial Hamiltonian $\hat{H}_0$, $\hat{c}^\dagger_k = \sum_\mu u^{0*}_{k\mu} \hat{c}^\dagger_\mu$ and $\hat{c}_k = \sum_\mu u^0_{k\mu} \hat{c}_\mu$ we get:

$$\delta^2_{j_1 j_2} \leq \frac{8}{L^2} \sum_{k_1 k_2} \sum_{\mu_1 \mu_2} u^{0*}_{k_1 \mu_1} u^0_{k_2 \mu_1} u^0_{k_1 \mu_2} u^{0*}_{k_2 \mu_2} n^0_{\mu_1} n^0_{\mu_2} = 8 \frac{N^0_{\mathrm{F}}}{L^2} \tag{5}$$

where $n^0_\mu = \langle\psi_0| \hat{c}^\dagger_\mu \hat{c}_\mu |\psi_0\rangle$ and $N^0_{\mathrm{F}} = \sum_\mu n^0_\mu$ is the total number of fermions in the initial state (the last equality follows from the orthonormality of the wave-functions).

## QUENCH WITH NON VANISHING OFF-DIAGONAL CORRELATIONS IN THE INITIAL $|\psi_0\rangle$

When the final Hamiltonian is homogeneous we can construct cases in which $G_{k_1k_2} = \langle\psi_0|\,\hat{c}^{\dagger}_{k_1}\hat{c}_{k_2}\,|\psi_0\rangle$ has important non-vanishing contributions also for $k_1 \neq k_2$. Here we present a very simple example. Let's consider an initial Hamiltonian $\hat{H}_0$ that has $J^x_j = J^y_j = 0$ everywhere, and has regular repeated intervals of size $M$ with positive and negative magnetic field $h_j$ (see sketch in the figure below). In essence, the initial state $|\psi_0\rangle$ is given by a set of fermions localized in the sites where $h^0_i$ is positive. The final Hamiltonian is a homogeneous XX chain. Calculating $G_{k_1k_2}$ we get:

$$G_{k_1k_2} = \frac{1}{L}\frac{\sin\left((k_1-k_2)L/2\right)}{\sin\left((k_1-k_2)M\right)}\frac{\sin\left(\frac{k_1-k_2}{2}M\right)}{\sin\left(\frac{k_1-k_2}{2}\right)} \tag{6}$$

which we plot in the inset of Fig. 1 for $M = 2$ and two different sizes. Clearly, the off-diagonal terms of $G_{k_1k_2}$ do not vanish in the thermodynamic limit, but reveal a well defined structure: a series of Kronecker's delta centered at $k_1 - k_2 = 2\pi m$ and $k_1 - k_2 = \pi(2m+1)/M$ with $m$ a natural number. In the main panel of figure 1 there is a plot of $\delta G_{j_1j_2}(t)$ and we see that the fluctuations go to zero with an envelope $1/\sqrt{t}$, confirming that, while $G_{k_1k_2}$ is not necessarily a simple delta-function $\delta_{k_1,k_2}$, the fluctuations still vanish when the final $\hat{H}$ is clean, independently of the initial state $|\psi_0\rangle$.

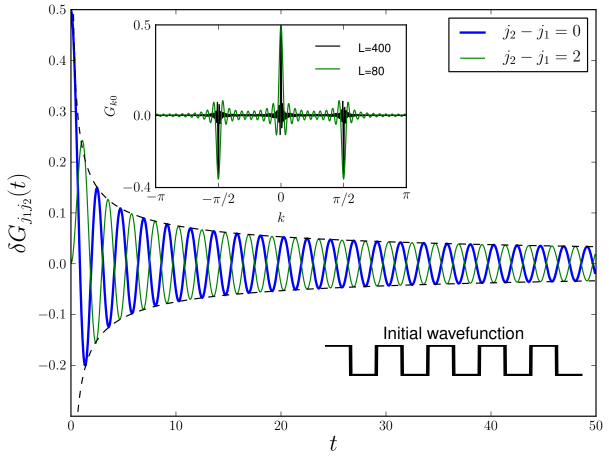


FIG. 1: Time fluctuations of $G_{j_1j_2}(t)$ for a quench of a XX chain with $L = 2000$. The final Hamiltonian is homogeneous with $h_f = 0.5$ and the initial $\hat{H}_0$ has $J^x_j = J^y_j = 0$ and $h^0_i$ grater than zero only on consecutive intervals of amplitude 2 (square wave pattern). The dashed line is the envelop $\pm 1/\sqrt{\sqrt{2}\pi J t}$. In the inset there are two plots of $G_{k_1k_2}$ with $k_2 = 0$, for the same quench, but two different sizes.

---

[1] This is due to the fact that the condition $\epsilon_{k_1} - \epsilon_{k_2} - \epsilon_{k_3} + \epsilon_{k_4} = 0$ is fulfilled only when $|k_3| = |k_1|$ and $|k_4| = |k_2|$ or when $|k_3| = \pi - |k_2|$ and $|k_4| = \pi - |k_1|$ (because of particle-hole symmetry). At fixed $k_1$ and $k_2$ there are 8 values of $k_3$ and $k_4$ with which $\Delta(k_1, k_2, k_3, k_4)$ is one. The cases in which the summation is 4 is instead due to the double counting happening when the two condition are both fulfilled.
